# Supplementary material for: Asymptotically-Optimal Multi-Query Path Planning for a Polygonal Robot
Source: arXiv:2409.03920 source file (2025-03-25)
Supplement: Supplementary file 1 [file 16-appendix.tex]

\ours is \emph{resolution complete} and \emph{asymptotically optimal}. 
Resolution completeness refers to the ability of a motion planning method to find a solution, if one exists, at a sufficiently high resolution\footnote{Note that there can be conflicting interpretations of \emph{high} resolution. Here, we use high resolution to refer to the high number of divisions, as is commonly used in, e.g., display resolution. One opposite interpretation of resolution (which is not what we use here) is measured by the dimensions of the smallest block, e.g., the smallest display cell size is at $x$-millimeters.}. 
In the context of this study, the $\delta$-clearance assumption expands any existing path to an ensemble of homotopic paths. The $\delta$-clearance assumption further implies that no obstacle may be enclosed by a ball with a radius of $\delta$. Therefore, there are no arbitrarily small polygonal obstacles in the environment.
In the context of this study, resolution completeness and asymptotic optimality are defined in Def~\ref{def:resolution_completeness} and Def~\ref{def:asymptotical_optimality}.

\begin{definition}[Resolution Completeness]
    \label{def:resolution_completeness} 
    For the problem defined in Sec.~\ref{subsec:prob}, if a solution exists, a resolution complete algorithm will find a solution in finite time, as the orientation resolution $n$ becomes sufficiently large.
\end{definition}

\begin{definition}[Asymptotic Optimality]
    \label{def:asymptotical_optimality}
    For the problem defined in Sec.~\ref{subsec:prob} and a fixed cost structure defined in Eq.~\eqref{eq:cost}, let $J^*$ be the infimum of the costs of all feasible solutions. An asymptotically optimal method can compute paths with costs arbitrary close to $J^*$ at sufficiently high resolution.
\end{definition}

\subsection{Topological traits of the optimal path in $SE(2)$}
To prove the asymptotic optimality, the basic topological traits of the optimal path need to be clarified. Given the robot and obstacles, the semi-algebraic sets are built in the $SE(2)$ space, and $\RVG$ are built upon the semi-algebraic sets according to Alg~\ref{alg:building_layers} and Alg~\ref{alg:propagation}. When the resolution tends to infinity, then the zero set of semi-algebraic sets becomes a set of continuous surfaces $\set{x | S_i(x)=0}$.
Thus, we formulate the shortest path problem in $SE(2)$ space as the following:
\begin{align}
        \tau^* = \argmin_{\tau}J(\tau) \quad
        s.t. \quad S_i(\tau(t)) \ge 0
\end{align}

With the cost function defined in Eq.~\ref{eq:cost}, the partial linearity of $\tau^*$ can be established in the following lemma:
\begin{lemma}[Piecewise Linearity]
   Assuming $\delta$-clearance, an optimal solution is piecewise linear.
\end{lemma}
\begin{proof}
    We prove this via contradiction. Assuming the optimal solution for a given instance is not linear at the parts in the free space or on the surface $S_i$, there are a few cases, none of which can happen:
    \begin{itemize}[leftmargin=4mm]
        \item If the curve is in the free space as shown in Fig~\ref{fig:linearity:a}, then two points on the curve whose connection is also in the free space can always be found, leading to a shortcut compared with the curve between the two points. For example, we can always take a sphere centered at any point on the curve with a radius of $\delta$, and the intersection between the sphere and the curve constructs a shortcut. 
        \item If the curve is on the obstacle and it's curved inwards to the surface, then any points on the curve are non-reflex, and none of them will be in the shortest path. A shortcut can be easily found by placing the $\delta$-sphere at any place of the curve and connecting the two intersections between the $\delta$-sphere and the curve as shown in Fig~\ref{fig:linearity:b}.
        \item If the curve is on the obstacle and it curves outwards as shown in Fig~\ref{fig:linearity:c}, it's a spiral curve in the $SE(2)$ space(refer to Fig~\ref{fig:semi-alge}) according to how the obstacles are grown in Alg~\ref{alg:building_layers}, where each point on it has different $\theta$.
        A shortcut can be easily found by placing the $\delta$-sphere at any place of the curve and connecting the two intersections between the $\delta$-sphere and the curve as shown in Fig~\ref{fig:linearity:c}.
    \end{itemize}
    Proved by contradiction.  
    \label{proof:linearity}
\end{proof}
% \jy{When would a shortest path segment contain a curve?}

\begin{figure}[h!]
\centering
\begin{subfigure}[b]{0.3\linewidth}
\frame{\includegraphics[width=\linewidth, trim=1.8cm 2cm 1.8cm 1.3cm, clip]{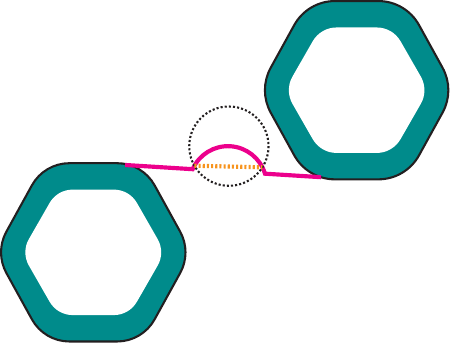}}
\caption{}
\label{fig:linearity:a}
\end{subfigure}
\begin{subfigure}[b]{0.3\linewidth}
\frame{\includegraphics[width=\linewidth, trim=1.4cm 2.12cm 1.6cm 1.3cm, clip]{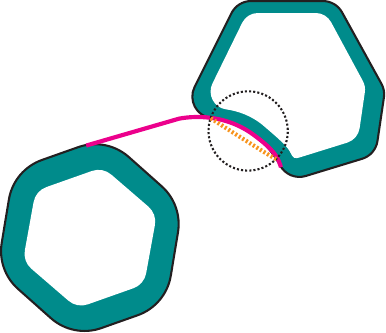}}
\caption{}
\label{fig:linearity:b}
\end{subfigure}
\begin{subfigure}[b]{0.3\linewidth}
\frame{\includegraphics[width=\linewidth, trim=2.5cm 1.35cm 1cm 0.75cm, clip]{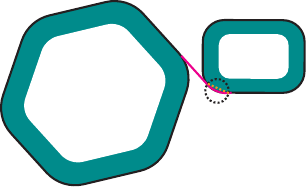}}
\caption{}
\label{fig:linearity:c}
\end{subfigure}
\caption{The possible cases of curved paths. The orange dotted lines, the magenta lines, the dark cyan shapes and the black dotted circle are, respectively, the shortcut, the assumed optimal path, the obstacle surface projected to $\mathbb{R}^2$ space and the $\delta$-sphere.}
\label{fig:linearity}
\end{figure}

\subsection{Convergence to the optimal path}
The optimal path comprises a set of straight line segments in the $SE(2)$ space, whose two ends are all reflex vertices. We will show that, for arbitrarily $\delta > 0$, all reflex vertices can be approximated close enough at sufficiently high resolutions. 
\begin{lemma}[Arbitrary Approximation of Reflex Vertices on $\set{S_i}$]
     Given a reflex vertex $v=(x, y, \theta)$ on $S_i$ and arbitrarily $\delta >0$, a resolution $\mathcal{N}$ can be always found that $\forall n>\mathcal{N}$, there is at least one reflex vertex $v'=(x', y', \theta')$ in $\RVG$ is in the $\delta$-sphere of $v$.
     \label{lemma:approximation}
\end{lemma}

\begin{proof}
    As shown in Fig~\ref{fig:approximation}, the red dot $v$ is a reflex vertex on $S_i$ where the red dotted line is the curve made of the continuous rotation of one vertex on the robot's geometry. 
    Given $\delta$, a resolution $\mathcal{N}$ and the alignment of the rotation range $\layerrange$ of the robot can always be found with the following criteria:
    \begin{itemize}[leftmargin=4mm]
        \item For all layers, $\Delta \theta = \lvert \theta_{ub}-\theta_{lb}\rvert = \frac{2\pi}{\mathcal{N}} \le 2\delta$ is satisfied.
        \item There are two consecutive layers that have rotation ranges of $[\theta-\Delta \theta, \theta]$ and $[\theta, \theta + \Delta\theta]$.
    \end{itemize}
    Thus, the same vertex on the robot's geometry approximated in two consecutive layers (The brown and black vertices right above and below the red dot shown in Fig~\ref{fig:approximation}) lie within the $\delta$-sphere round $v$.
    To conclude, when $n$ satisfy the following inequality:
    \begin{align}
        n>\mathcal{N}=\frac{\pi}{\delta}   
        \label{eq:find_N}
    \end{align}
    a reflex vertex $v$ on $\set{S_i}$ can be approximated within the $\delta$-sphere around $v$.
\end{proof}

\begin{figure}[h!]
\centering
\includegraphics[width=0.3\linewidth, trim=5cm 4cm 7.5cm 7cm, clip]{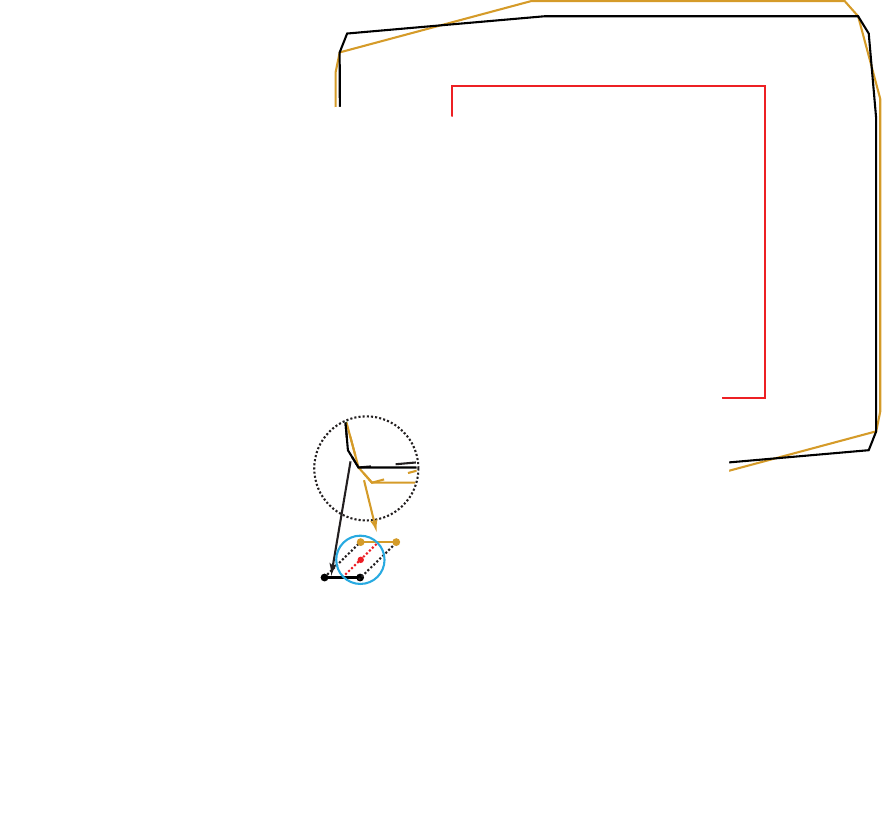}
\caption{An illustration of how a reflex vertex on $S_i$ is approximated by \ours using the example's bottom left corner in Fig~\ref{fig:minkowski_sum}. The red dot is one of the reflex vertexes to be approximated; the red dotted line is the reflex vertices generated from the Minkowski sum between one of the corners of the obstacle and the robot geometry at different angles and the blue circle is the $\delta$-sphere around the reflex vertex.}
\label{fig:approximation}
\end{figure}

Because all reflex vertices on $\set{S_i}$ can be well approximated, \ours produces asymptotically optimal solutions. 
\begin{theorem}[Asymptotical Optimality]
    \ours is asymptotically optimal according to Def~\ref{def:asymptotical_optimality}.
\end{theorem}
\begin{proof}
    By Lemma~\ref{lemma:approximation}, any two neighboring reflex vertices $v_1, v_2$ on the optimal path can be arbitrarily approximated given $\delta$, while the connection between them indicates the visibility. Thus, while building $\RVG$, all the approximations of $v_1, v_2$ are connected because they are visible reflex vertices. Then an approximation within the $\delta$-clearance of the optimal path can be found by the shortest path search in $\RVG$ based on Eq.~\ref{eq:cost}.
    
    To argue the visibility between the approximations of $v_1, v_2$, we can assume that all the approximations of $v_1, v_2$ are not visible to each other no matter how small the value $\delta$ takes, then it means there's an obstacle in between whose size can be upper bounded by $\delta$, leading to contradiction.

    At last, according to Eq.~\ref{eq:find_N}, we have $\lim_{n\to \infty} \delta =0$.
    \label{proof:asymptotical_optimality}
\end{proof}
\begin{theorem}[Resolution Completeness]
   \ours is resolution complete according to Def~\ref{def:resolution_completeness}.
\end{theorem}
\begin{proof}
    By Theorem~\ref{proof:asymptotical_optimality}, \ours converges to the optimal solution, thus given $\delta$, we can at least find a solution after $n>\mathcal{N}$ where $\mathcal{N}$ can be determined in \ref{lemma:approximation}.
\end{proof}

\subsection{Complexity Analysis}
We now examine the complexity of \ours. Let $n$ denote the resolution, $k$ represent the total number of obstacles in a given problem instance, and $m$ the total number of vertices (equal to the number of edges), including the polygonal environment and the robot.

\subsubsection{Complexity for building layers}
By \cite{bungiu2014efficient}, computing the visible area for a vertex in a polygonal environment comprises preprocessing and query. For preprocessing, the polygonal environment will be triangulated, which takes $O(m)$ time. The query will be done with $O(mk)$ (Triangular Expansion). Checking whether a vertex is inside another vertex's visible area and connects them takes $O(m)$ time. However, this can be sped up using Bounding Volume Hierarchy(BVH) or KD-Tree.
Since such a process needs to be done for all the vertices in one layer, the complexity of building the visibility graph for one layer is $O(m^2k)$, leading to a $O(nm^2k)$ complexity for building all layers. 

\subsubsection{Vertex Propagation}
While doing vertex propagation between 2 layers, all the vertices at the current layer need to be checked to see whether they are in any visible areas of the vertices in the next layer. Also, all vertices in the current layer could potentially be added to the next layer. Thus, there could be at most $O(nm)$ checks, leading to a $O(nm^2)$ complexity.

\subsubsection{Query Path Given Start and Goal Configuration}
The visible areas of the start and the goal in each layer should be calculated, which takes $O(nmk)$ time.

The analysis indicates that layer-building efforts dominate the overall computation time. The overall computational complexity is $O(nm^2k)$.
